# Supplementary material for: Faster Algorithms for Growing Collision-Free Convex Polytopes in Robot Configuration Space
Source: arXiv:2410.12649 source file (2024-11-13)
Supplement: Supplementary file 1 [file proofs.tex]

\section{Proofs}\label{app:proofs}

\textbf{Proof} Observe that $\Prob\left[\bar X_N'  \le (1-\tau) p \right] \le \Prob\left[\bar X_N'  \le (1-\tau) p' \right]$. If $\tau>1$ both sides evaluate to 0, and otherwise $(1-\tau) p \leq (1-\tau) p'$. Next, we use the standard multiplicative concentration bound, $\Prob\left[\bar X_N'  \le (1-\tau) p' \right]\leq e^{-Np'\tau^2/2},$ 
e.g. given in \cite[\S A, Thm A.1.15]{alon2016probabilistic}, and use the fact that $e^{-Np'\tau^2/2} \le  e^{-Np\tau^2/2}$. We have now shown that $\Prob\left[\bar X_N'  \le (1-\tau) p \right]\leq e^{-Np\tau^2/2}$, and the final result follows from evaluating $N = 2 \log(1/\delta)/p \tau^2$.\qed

\noindent\textbf{Proof Corollary 1}

\textbf{Proof} We have $\Prob\left[\bar{X}_N>(1-\tau)p'\right] = 1 - \Prob\left[\bar{X}_N\leq(1-\tau)p'\right]\geq1-\delta.$\qed

% \begin{lemma}[Muliplicative Concentration Inequality]\cite[\S A, Thm A.1.15]{alon2016probabilistic}

%     Let $(X_i)_{i\geq1}\sim\mathrm{Bernoulli}(p)$, and let $N$ be fixed. Define $\bar X_N:=\frac{1}{N}\sum_{i=1}^NX_i$. Then, for any fixed parameter $\tau>0$, 
%     \begin{gather}
%         \Prob\left[\bar X_N \leq(1-\tau)p\right]\leq e^{-Np\tau^2/2}.
%     \end{gather}
% \end{lemma}

% As a direct consequence we get Corollary \ref{cor:samps}.

% \begin{corollary}[Sample Bound]\label{cor:samps} 

% For $p' \ge p$, let $(X_i')_{i \ge 1} \sim \mathrm{Bernoulli}(p')$. Then, 
% \begin{align}
%     \Prob\left[\bar X_N'  \le (1-\tau) p \right] \le e^{-Np\tau^2/2}.
% \end{align}
% Hence, with $N = 2\log(1/\delta)/p\tau^2$ samples, if $(X_i')_{i \ge 1} \sim \mathrm{Bernoulli}(p')$, and $p' \ge p$, as well as $\delta\in(0,1]$, we have 
% \begin{align}
%     \Prob\left[ \bar X_N' \le (1-\tau)p\right]\le \delta. 
% \end{align}
% \end{corollary}
% \textbf{Proof}
%     $\Prob\left[\bar X_N  \le (1-\tau) p \right] \le \Prob\left[\bar X_N  \le (1-\tau) p' \right]  \le e^{-Np'\tau^2/2} \le  e^{-Np\tau^2/2}$, and the second result follows by evaluation. \qed
