# Supplementary material for: Faster Algorithms for Growing Collision-Free Convex Polytopes in Robot Configuration Space
Source: arXiv:2410.12649 source file (2024-11-13)
Supplement: Supplementary file 2 [file unadaptivetest.tex]

\section{Statistical Power of Unadaptive Test}\label{app:unadapt}

\pwcomment{TODO}
